# Supplementary material for: On the Expansion of Group-Based Lifts
Source: arXiv:1311.3268 source file (2016-12-17)
Supplement: Supplementary file 1 [file appendix.tex]

\section*{Appendix}
